# Supplementary material for: Character Region Attention For Text Spotting
Source: arXiv:2007.09629 source file (2020-07-19)
Supplement: Supplementary file 1 [file 6-Appendix.tex]

%\section*{Supplemental materials}
\section{\textit{LinkRefiner} for CTW-1500 dataset}

\begin{figure}[h]
	\begin{center}
        \includegraphics*[width=0.8\linewidth, clip=true]{fig/architecture_refiner}
         \vspace{+1mm}
        \caption{Schematic illustration of \textit{LinkRefiner} architecture.}
  	    \label{fig:architecture_refiner} 
    \end{center}
     \vspace{-1.5mm}
\end{figure}

CTW-1500 dataset~\cite{yuliang2017detecting} provides polygon-only annotations without text transcriptions. %The CRAFT model cannot be directly trained on CTW-1500 due to these properties. 
Furthermore, annotations of CTW-1500 are provided at the line-level and does not consider spaces as separation cues. This is far from our assumption of affinity, which is that the score for affinity is zero for characters with a space between them.

To obtain a single-long polygon from the detected characters, we employ a shallow network for link refinement,  so called \textit{LinkRefiner}. The architecture of the \textit{LinkRefiner} is shown in Fig.~\ref{fig:architecture_refiner}. The input of the \textit{LinkRefiner} is a concatenation of the \textit{region score}, the \textit{affinity score}, and the intermediate feature map from the network, that is the output of \textit{Stage4} of the original CRAFT model. Atrous Spatial Pyramid Pooling (ASPP) in \cite{chen2018deeplab} is adopted to ensure a large receptive field for combining distant characters and words onto the same text line.

For the ground truth of the \textit{LinkRefiner}, lines are simply drawn between the centers of the paired control points of the annotated polygons, which is similar to the text line generation used in \cite{he2016accurate}. The width of each line is proportional to the distance between paired control points. The ground truth generation for the \textit{LinkRefiner} is illustrated in Fig.~\ref{fig:gt_generation_refiner}. The output of the model is called the \textit{link score}. For training, only the \textit{LinkRefiner} is trained on the CTW-1500 training dataset, while freezing CRAFT.
%Empirically, we adjust the width as 1/10 of diagonal length.

After training, we have the outputs produced by the model, which are the \textit{region score}, the \textit{affinity score}, and the \textit{link score}. Here, the  \textit{link score} is used instead of the original \textit{affinity score}, and the text polygon is obtained entirely through the same process as done with TotalText. The CRAFT model localizes the individual characters, and the \textit{LinkRefiner} model combines the characters as well as the words separated by spaces, which are required by the CTW-1500 evaluation.

\begin{figure}[t]
	\begin{center}
        \includegraphics*[width=0.8\linewidth, clip=true]{fig/gt_generation_refiner}
        \caption{Ground truth generation for \textit{LinkRefiner}.}
  	    \label{fig:gt_generation_refiner} 
    \end{center}
    \vspace{-1.5mm}
\end{figure}

The results on the CTW-1500 dataset are shown in Fig.~\ref{fig:result_ctw}. Very challenging image samples with long and curved texts are successfully detected by the proposed method. Moreover, with our polygon representation, the curved images can be rectified into straight text images, which are also shown in Fig.~\ref{fig:result_ctw}. We believe this ability for rectification can further be of use for recognition tasks.

\begin{figure*}[t]
  \centering
  \includegraphics*[width=16.5cm, clip=true]{fig/result_ctw.jpg}
  \caption{Results on CTW-1500 dataset. For each cluster: the input image (top), region score (middle left), link score (middle right), and the resulting rectified polygons for curved texts (bottom, below arrow) are shown. Note that the affinity scores are not rendered and are unused in the CTW-1500 dataset.} 
  \label{fig:result_ctw} 
\end{figure*}
